# Supplementary material for: RemovalNet: DNN Fingerprint Removal Attacks
Source: arXiv:2308.12319 source file (2023-11-22)
Supplement: Supplementary file 1 [file Appendix.tex]

\appendix

\section{External code source}
\begin{table}[!ht]
    \centering
    \caption{Sources of codes used for experiments from external}
    \begin{tabular}{|c|c|}
    \hline
    Task & Code Source \\
    \hline
    ModelDiff ~\cite{li2021modeldiff} & \url{https://github.com/yuanchun-li/ModelDiff} \\
    \hline
    DeepJudge ~\cite{chen2022copy} & \url{https://github.com/Testing4AI/DeepJudge} \\
    \hline
    ZEST ~\cite{jia2021zest} & \url{https://github.com/cleverhans-lab/Zest-Model-Distance} \\
    \hline
    Sensitive-Sample ~\cite{he2019sensitive} & \url{https://github.com/oaramoon/SensitiveSamples-TensorFlow} \\
    \hline
    Dataset Inference ~\cite{pratyush2021dataset} & \url{https://github.com/cleverhans-lab/dataset-inference} \\
    \hline
    MetaFinger~\cite{yang2022metafinger} & 
    \url{https://github.com/kangyangWHU/MetaFinger} \\
    \hline
    \end{tabular}
\end{table}

\subsection{Experiments Setting}

\textbf{MetaFinger}

For train data, we use
